# Supplementary material for: Semantic Hierarchy Emerges in Deep Generative Representations for Scene Synthesis
Source: arXiv:1911.09267 source file (2020-02-11)
Supplement: Supplementary file 1 [file appendix.tex]

% !TEX root = main.tex


% According to our experimental results, \emph{layout}, \emph{object (category)}, \emph{attribute}, \emph{color scheme} correspond to \emph{bottom}, \emph{lower}, \emph{upper}, and \emph{top} layers respectively, which are actually $\left[0,2\right)$, $\left[2,6\right)$, $\left[6,12\right)$ and $\left[12, 14\right)$ layers.
% %
% As for BigGAN model with $256\times256$ resolution, there are total 12 convolutional layers.
% %
% As the category information is already encoded in the ``class'' code as shown in Fig.\ref{fig:structure}, we only separate the layers to two groups, which are \emph{lower} (bottom 6 layers) and \emph{upper} (top 6 layers).
% %
% Since our layout model can only be applied to indoor scenes yet the BigGAN model is trained on Places dataset which contains both indoor and outdoor categories, we only analyze BigGAN from attribute level as shown in Fig.\ref{fig:other-models}(b).
% %
% Both visualization results and quantitative curve suggest that attribute-level semantics are better controlled by \emph{upper} layers of BigGAN.
% %
% For example, when manipulating ``vegetation'' attribute at lower layers or all layers, the spatial information varies unexpectedly, while manipulating at upper layers gives desired output.
% %



% \begin{figure*}[t]
%   \centering
%   \includegraphics[width=0.8\textwidth]{figures/layout_category.pdf}
%   \captionsetup{font=small}
%   \caption{
%     Layout and objects manipulation results.
%   }
%   \label{fig:layout-category}
% \end{figure*}





% \begin{figure*}[t]
%   \centering
%   \includegraphics[width=0.95\textwidth]{figures/joint.pdf}
%   \vspace{-15pt}
%   \captionsetup{font=small}
%   \caption{
%     Independent and joint manipulation results.
%   }
%   \label{fig:joint}
% \end{figure*}
